# Supplementary material for: Overcoming the Long Horizon Barrier for Sample-Efficient Reinforcement Learning with Latent Low-Rank Structure
Source: arXiv:2206.03569 source file (2023-06-09)
Supplement: Supplementary file 1 [file algorithm_pseudocode.tex]

\section{Algorithm Pseudocode}\label{sec:pseudo}

%empirical value iteration; does a bellman update; backwards recursion over the horizon; but modification ...
%standard value iteration update is
%V_h(s) = \max_a \sum_s' P(s'| s a) (R(s,a,') + V_{h+1}(s'))
%This involves evaluating Q at all s,a, which involves an expectation wrt P(s' | sa); could be data costly. We use matrix estimation to approximate this step
In this section, we present the pseudocode of our main algorithm, Algorithm \ref{alg:1}. LR-EVI is Algorithm \ref{alg:1} with \texttt{Qestimate}$=$\texttt{transition}, and LR-MCPI is Algorithm \ref{alg:1} with \texttt{Qestimate}$=$\texttt{trajectory}.

\begin{algorithm}[H]
\caption{ }\label{alg:1}
\hspace*{\algorithmicindent} \textbf{Input:} $S, A, H, \{N_h, N_h^{\#}\}_{h=1,\ldots, H}, p_1, p_2,\hat{V}_{H+1} = \Vec{0},$ $\hat{\pi}_{H+1} = \text{ uniform}(A)$, and \texttt{Qestimate}$(\cdot, \cdot, \cdot, \cdot, \cdot)$ 
\\
\hspace*{\algorithmicindent} \textbf{Output:} $\hat{\pi} = \{\hat{\pi}_h\}_{h=1,\ldots, H}$ and $\{\bar{Q}_h\}_{h\in [H}$
\begin{algorithmic}[1]
\For{$t = 0, \ldots, H-1$}
\State $/*$ Step 1: Build the sets of anchor states and actions according to $p_1$ and $p_2$, respectively.
\State Sample $B_i^S \sim Bernoulli(p_1)$ and $B_j^A \sim Bernoulli(p_2)$ for $i \in [|S|], j \in [|A|]$.
\State Define the anchor states and actions as:
\[
S^\# \xleftarrow[]{} \{s_i \in S \mid B_i^S = 1\}, \quad A^\# \xleftarrow[]{} \{a_j \in A \mid B_j^A = 1\}
\]
    \State $/*$ Step 2: Compute $\hat{Q}_{H-t}$ over $\Omega_{H-t}= \{(s,a) \in S \times A \mid s \in S^{\#} \text{ or } a \in A^{\#}\}$ to use the matrix estimation method to obtain an estimate of $Q^*_{H-t},Q^{\hat{\pi}}_{H-t},$ or $r_{H-t} + [P_{H-t}\bar{V}_{H-t}]$. 
\For{$(s, a) \in \Omega_{H-t}^{\#} = S^{\#} \times A^{\#}$}
    \State Estimate $Q^*_{H-t}, Q^{\hat{\pi}}_{H-t},$ or $r_{H-t} + [P_{H-t}\bar{V}_{H-t}]$ by calling \texttt{QEstimate}$(\hat{\pi}_{H-t+1}, \bar{V}_{H-t+1}, (s,a), N_{H-t},  H-t)$:
    \[
        \hat{Q}_{H-t}(s, a) \xleftarrow{}  \mathrm{\texttt{QEstimate}}(\hat{\pi}_{H-t+1}, \bar{V}_{H-t+1}, (s,a), N_{H-t}^{\#},  H-t)
    \]
    where $\hat{\pi}_{H-t+1} = \{\hat{\pi}_h\}_{H-t +1 \leq h \leq H}$. 
\EndFor
\For{$(s, a) \in \Omega_{H-t}\setminus \Omega_{H-t}^{\#}$}
    \State Estimate $Q^*_{H-t}, Q^{\hat{\pi}}_{H-t},$ or $r_{H-t} + [P_{H-t}\bar{V}_{H-t}]$ by calling \texttt{QEstimate}$(\hat{\pi}_{H-t+1}, \bar{V}_{H-t+1}, (s,a), N_{H-t},  H-t)$:
    \[
        \hat{Q}_{H-t}(s, a) \xleftarrow{}  \mathrm{\texttt{QEstimate}}(\hat{\pi}_{H-t+1}, \bar{V}_{H-t+1}, (s,a), N_{H-t},  H-t)
    \]
    where $\hat{\pi}_{H-t+1} = \{\hat{\pi}_h\}_{H-t +1 \leq h \leq H}$. 
\EndFor
\State $/*$ Step 3: Use the matrix estimation method to obtain $\bar{Q}_{H-t}$ over $S\times A$ from $\hat{Q}_{H-t}$ over $\Omega_{H-t}$. 
\State Using the low-rank structure of $Q^*_{H-t}, Q^{\hat{\pi}}_{H-t},$ or $r_{H-t} + [P_{H-t}\bar{V}_{H-t}]$, produce an estimate with:
\[
\bar{Q}_{H-t}(s, a) \xleftarrow{} \hat{Q}_{H-t}(s,A^{\#})[\hat{Q}_{H-t}(S^{\#}, A^{\#})]^\dagger\hat{Q}_{H-t}(S^{\#}, a)
\]
\State $/*$ Step 4: Identify the optimal action for each state at time step $H-t$ to build our policy and compute $\bar{V}_{H-t}$ by greedily choosing actions using $\bar{Q}_{H-t}$.
\For{$s \in S$}
\State Determine the optimal action via $\bar{Q}_{H-t}(s, a)$:
\[
\hat{\pi}_{H-t}(s) \xleftarrow{} \argmax_{a \in A} \bar{Q}_{H-t}(s, a)
\]
\State Compute the optimal value function estimate:
\[
\bar{V}_{H-t}(s) \xleftarrow{} \max_{a \in A} \bar{Q}_{H-t}(s, a)
\]
\EndFor
\EndFor
\end{algorithmic}
\end{algorithm}

\begin{algorithm}[H]
\caption{\texttt{trajectory}$(\cdot, \cdot, \cdot, \cdot, \cdot)$ }\label{alg:roll}
\hspace*{\algorithmicindent} \textbf{Input:} $\hat{\pi}_{H-t+1}, \bar{V}_{H-t+1}, (s,a), N_{H-t}, \text{ and } H-t$\\
\hspace*{\algorithmicindent} \textbf{Output:} $Q^\mu_{H-t}(s,a)$
\begin{algorithmic}[1]
\State Initialization: $s_{H-t} \leftarrow s, a_{H-t} \leftarrow a, $ and $Q^\mu_{H-t}(s,a) \leftarrow 0$.
\For{$j = 1, \ldots, N_{H-t}$}
\State $/*$ Obtain the reward of a trajectory following $\hat{\pi}_{H-t+1}$ starting at state $(s,a)$ at step $H-t$.
\State $\hat{Q}_{H-t}(s,a) \sim R_{H-t}(s_{H-t},a_{H-t})$.
\For{$i = H-t + 1, \ldots, H$}
\State Sample the next state: $s_{i} \sim P_{i}(\cdot|s_{i-1}, a_{i-1})$.
\State Sample the reward obtained at the next state following $\hat{\pi}_i$: $r'_i \sim R_i(s_i, \hat{\pi}_i(s_i))$:
\[
\hat{Q}_{H-t}(s,a) \leftarrow \hat{Q}_{H-t}(s,a)+ r'_i.
\]
\EndFor
\State Update the estimate:
\[
Q^\mu_{H-t}(s,a) \leftarrow Q^\mu_{H-t}(s,a) + \frac{\hat{Q}_{H-t}(s,a) }{N_{H-t}}
\]
\EndFor
\end{algorithmic}
\end{algorithm}

\begin{algorithm}[H]
\caption{\texttt{transition}$(\cdot, \cdot, \cdot, \cdot, \cdot)$ }\label{alg:transition}
\hspace*{\algorithmicindent} \textbf{Input:} $\hat{\pi}_{H-t+1}, \bar{V}_{H-t+1}, (s,a), N_{H-t}, \text{ and } H-t$\\
\hspace*{\algorithmicindent} \textbf{Output:} $Q^\mu_{H-t}(s,a)$
\begin{algorithmic}[1]
\State Initialization: $Q^\mu_{H-t}(s,a) \leftarrow 0$.
\For{$t = 1, \ldots, N_{H-t}$}
\State $/*$ Obtain the expected reward of a single transition starting at state $(s,a)$ at step $H-t$ with $\bar{V}_{H-t+1}$.
\State $\hat{Q}_{H-t}(s,a) \sim R_{H-t}(s_{H-t},a_{H-t})$.
\State Sample the next state: $s' \sim P_{H-t}(\cdot|s, a)$.
\State Update the estimate:
\[
Q^\mu_{H-t}(s,a) \leftarrow Q^\mu_{H-t}(s,a) + \frac{\hat{Q}_{H-t}(s,a) + \bar{V}_{H-t+1}(s') }{N_{H-t}}
\]
\EndFor
\end{algorithmic}
\end{algorithm}
