# Supplementary material for: Overcoming the Long Horizon Barrier for Sample-Efficient Reinforcement Learning with Latent Low-Rank Structure
Source: arXiv:2206.03569 source file (2023-06-09)
Supplement: Supplementary file 2 [file exponential_unique.tex]

\section{Yet Another MDP}
\label{sec:yet_another_mdp}

Fix $\alpha\in(0,1)$. Suppose $V_{H}=\left(\begin{array}{c}
\alpha\\
1
\end{array}\right)$, $P_{h}(\cdot|s,a)=\delta_{s}$, and $R_{h}=\left(\begin{array}{cc}
\alpha^{2}-\alpha & 0\\
\alpha-1 & 0
\end{array}\right),\forall h\in[H-1]$. Consider the policy 
\[
\pi_{h}(1)=\pi_{h}(2)=2,\qquad\forall h\in[H-1].
\]
The true value and Q functions of $\pi$ satisfy
\begin{align*}
Q_{h}^{\pi} & =R_{h}+P_{h}V_{h+1}=R_{h}+\left(\begin{array}{cc}
V_{h+1}^{\pi}(1) & V_{h+1}^{\pi}(1)\\
V_{h+1}^{\pi}(2) & V_{h+1}^{\pi}(2)
\end{array}\right)=\left(\begin{array}{cc}
\alpha^{2}-\alpha & 0\\
\alpha-1 & 0
\end{array}\right)+\left(\begin{array}{cc}
\alpha & \alpha\\
1 & 1
\end{array}\right)=\left(\begin{array}{cc}
\alpha^{2} & \alpha\\
\alpha & 1
\end{array}\right),\\
V_{h}^{\pi} & =\left(\begin{array}{c}
Q_{h}^{\pi}\left(1,\pi_{h}(1)\right)\\
Q_{h}^{\pi}\left(2,\pi_{h}(2)\right)
\end{array}\right)=\left(\begin{array}{c}
Q_{h}^{\pi}\left(1,2\right)\\
Q_{h}^{\pi}\left(2,2\right)
\end{array}\right)=\left(\begin{array}{c}
\alpha\\
1
\end{array}\right),
\end{align*}
for all $h\in[H-1]$. Moreover, $\pi$ is the unique greedy policy
w.r.t.~$Q_{h}^{\pi}$, hence $\pi$ is the \textbf{(unique?)} optimal
policy.

Now suppose we have a noisy estimate of the terminal value function,
$\hat{V}_{H}^{\pi}=\left(\begin{array}{c}
\alpha\\
1+2\epsilon_{H}
\end{array}\right),$ where $\epsilon_{H}>0$. We compute estimates of the entries $Q_{h}^{\pi}(1,1),Q_{h}^{\pi}(1,2),Q_{h}^{\pi}(2,1)$
by applying the exact Bellman operator:
\begin{align*}
\hat{Q}_{h}^{\pi} & =R_{h}+P_{h}\hat{V}_{h+1}^{\pi}=R_{h}+\left(\begin{array}{cc}
\hat{V}_{h+1}^{\pi}(1) & \hat{V}_{h+1}^{\pi}(1)\\
\hat{V}_{h+1}^{\pi}(2) & \hat{V}_{h+1}^{\pi}(2)
\end{array}\right)\\
 & =\left(\begin{array}{cc}
\alpha^{2}-\alpha & 0\\
\alpha-1 & ?
\end{array}\right)+\left(\begin{array}{cc}
\alpha & \alpha\\
1+2\epsilon_{h+1} & ?
\end{array}\right)\\
 & =\left(\begin{array}{cc}
\alpha^{2} & \alpha\\
\alpha+2\epsilon_{h+1} & ?
\end{array}\right).
\end{align*}
We then estimate the entry $Q_{h}^{\pi}(2,2)$ via ME: 
\[
\hat{Q}_{h}^{\pi}(2,2)=\frac{\hat{Q}_{h}^{\pi}(1,2)\cdot\hat{Q}_{h}^{\pi}(2,1)}{\hat{Q}_{h}^{\pi}(2,2)}=\frac{\alpha(\alpha+2\epsilon_{h+1})}{\alpha^{2}}=1+\frac{2}{\alpha}\epsilon_{h+1}.
\]
It follows that 
\[
\hat{V}_{h}^{\pi}=\left(\begin{array}{c}
\hat{Q}_{h}^{\pi}\left(1,\pi_{h}(1)\right)\\
\hat{Q}_{h}^{\pi}\left(2,\pi_{h}(2)\right)
\end{array}\right)=\left(\begin{array}{c}
\hat{Q}_{h}^{\pi}\left(1,2\right)\\
\hat{Q}_{h}^{\pi}\left(2,2\right)
\end{array}\right)=\left(\begin{array}{c}
\alpha\\
1+\frac{2}{\alpha}\epsilon_{h+1}
\end{array}\right)=:\left(\begin{array}{c}
\alpha\\
1+2\epsilon_{h}
\end{array}\right).
\]
Therefore, we have the error recursion
\[
\epsilon_{h}=\frac{1}{\alpha}\epsilon_{h+1},
\]
in which case $\epsilon_{h}$ remains positive and grows exponentially
in $H-h$ when $\alpha<1$.

Also note that $\pi_{h}(1)=\pi_{h}(2)=2$ is still the unique greedy
policy under the estimate $\hat{Q}_{h}^{\pi}$, since 
\begin{align*}
\hat{Q}_{h}^{\pi}(1,2) & =\alpha>\alpha^{2}=\hat{Q}_{h}^{\pi}(1,1),\\
\hat{Q}_{h}^{\pi}(2,2) & =1+\frac{2}{\alpha}\epsilon_{h+1}>\alpha+2\epsilon_{h+1}=\hat{Q}_{h}^{\pi}(2,1),
\end{align*}
where the last inequality holds because $0<\alpha<1$ and $\epsilon_{h+1}>0$.

\subsection{Restated as an information theoretical result}

From the above example, we can derive a sample complexity lower bound
for all algorithms. The idea is the following: We construct two low
rank MDPs with terminal value/reward functions $V_{H}=\left(\begin{array}{c}
\alpha\\
1+2^{-H}\epsilon
\end{array}\right)$ and $V_{H}=\left(\begin{array}{c}
\alpha\\
1-2^{-H}\epsilon
\end{array}\right)$, respectively. Regardless of the algorithm used, if one cannot distinguish
these two MDPs, then an $\epsilon$ error will be incurred in estimating
$V_{1}$. Moreover, if only noisy samples are given for $V_{H}$,
then one needs an exponentially large sample size to distinguish these
two MDPs.

\paragraph{Problem class:}

Consider a class of $H$-horizon MDP $M^{\theta}=(S,A,R^{\theta},P)$
indexed by $\theta$, where $S=A=[1,2]$, 
\[
R_{H}^{\theta}=\left(\begin{array}{c}
\frac{1}{2}\\
1+2\theta
\end{array}\right),\qquad R_{h}^{\theta}=\left(\begin{array}{cc}
-\frac{1}{4} & 0\\
-\frac{1}{2} & 2^{H-h}\theta
\end{array}\right),\qquad\text{and }P_{h}(\cdot|s,a)=\delta_{s},\qquad\forall s,a,\forall h\in[H-1].
\]
 There is also an $h=0$ step with a fixed initial state $s_{0}$,
where 
\[
R_{0}^{\theta}(s_{0},a)=0\qquad\text{and}\qquad P_{0}(\cdot|s_{0},a)=\delta_{a},\qquad\forall a\in A.
\]
We assume that $\theta\in\{\theta_{1},\theta_{2}\}$ takes on two
possible values, $\theta_{1}=-\frac{3}{4\cdot2^{H}}$ and $\theta_{2}=\frac{3}{4\cdot2^{H}}$.

This problem class corresponds to taking $\alpha=\frac{1}{2}$ in
the previous example. Note that if action $a=1$ (resp., $2$) is
taken at $h=0$, then the MDP will transition to state $1$ (resp.,
$2$) and then stay at this state in all subsequent steps. Below we
will show that the optimal $Q$ functions of this MDP is rank-1, for
both values of $\theta$.

\paragraph{Observation model:}

The learner observes $P_{h}$, $R_{H}^{\theta}(1)$, $R_{h}^{\theta}(s,a)$
for all $(s,a)\in\Omega:=\{(1,1),(1,2),(2,1)\}$ and $h\in[H-1]$.
That is, everything is precisely known except for quantities involving
$\theta$. In addition, the learner is given $n$ iid data points
$\{r_{i}:i\in[n]\}$, such that $r_{i}$ is Gaussian with mean equal
to $R_{H}^{\theta}(2)=1+2\theta$ and variance equal to 1.

One can interpret the observation model as follows: The learner has
infinitely many samples of the form $(s,a,s')$ for each $(s,a)$,
so $P_{h}$ can be estimated with zero error. Similarly, the learner
has infinitely many samples from $R_{H}(1)$ and $R_{h}(s,a)$ for
$(s,a)\in\Omega$. However, the learner cannot observe $R_{h}(2,2)$
and hence must estimate $Q_{h}(2,2)$ using the low-rank structure.
Finally, $n$ noisy observations of $R_{H}(2)$ is given. \\

Consider a deterministic policy $\pi$ given by $\pi_{h}(1)=\pi_{h}(2)=2,h\in[H-1]$.
For both $\theta\in\{\theta_{1},\theta_{2}\}$, a similar calculation
as before shows that the true value and Q functions of $\pi$ are
\[
Q_{h}^{\theta}=\left(\begin{array}{cc}
\frac{1}{4} & \frac{1}{2}\\
\frac{1}{2}+2^{H-h}\theta, & 1+2^{H-h+1}\theta
\end{array}\right),\qquad V_{h}^{\theta}=\left(\begin{array}{c}
\frac{1}{2}\\
1+2^{H-h+1}\theta
\end{array}\right),\qquad h=1,\ldots,H-1.
\]
Moreover, since $2^{H}|\theta|=\frac{3}{4}<1$, we have $Q_{h}^{\theta}(2,2)=2\cdot Q_{h}^{\theta}(2,1)>0,\forall h\in[H-1]$
and hence $\pi$ is the unique optimal policy for $h\ge1$. Finally,
note that $Q_{h}^{\theta}$ has rank 1 for all $h\in[H-1]$.

Turning to step $h=0$, we observe that:
\begin{itemize}
\item If $\theta=\theta_{1}$, then $V_{1}^{\theta}(1)=\frac{1}{2}>\frac{1}{4}=V_{1}^{\theta}(2)$
, in which case the optimal policy for step $h=0$ is $\pi_{0}(s_{0})=1$
(``go to state 1'') with optimal value $V_{0}^{\theta}(s_{0})=V_{1}^{\theta}(1)=\frac{1}{2}$.
For the suboptimal policy $\pi_{0}(s_{0})=2$, its value is $V_{1}^{\theta}(2)=\frac{1}{4}$
with a suboptimality gap $\frac{1}{4}$.\footnote{There are other suboptimal policies that are stochastic. The argument
in this section can be generalized to stochastic policies.}
\item If $\theta=\theta_{2}$, $V_{1}^{\theta}(1)=\frac{1}{2}<\frac{7}{4}=V_{1}^{\theta}(2)$,
hence the optimal policy is $\pi_{0}(s_{0})=2$ with optimal value
$V_{0}^{\theta}(s_{0})=V_{h}^{\theta}(2)=\frac{7}{4}$. The suboptimal
policy $\pi_{0}(s_{0})=1$ has value $V_{1}^{\theta}(1)=\frac{1}{2}$
with a suboptimality gap $\frac{5}{4}$.
\end{itemize}
Therefore, to find a $\frac{1}{8}$-suboptimal policy, the learner
must correctly determine whether $\theta=\theta_{1}$ or $\theta=\theta_{2}$
from the data $\{r_{i}\}_{i\in[n]}$. This is a binary hypothesis
testing problem. Standard argument (e.g., Le Cam's method) shows that
learner needs a sample size at least 
\[
n\gtrsim\frac{1}{(2\theta_{1}-2\theta_{2})^{2}}=\frac{4^{H}}{9},
\]
which is exponentially large in $H$.
