# Supplementary material for: Overcoming the Long Horizon Barrier for Sample-Efficient Reinforcement Learning with Latent Low-Rank Structure
Source: arXiv:2206.03569 source file (2023-06-09)
Supplement: Supplementary file 3 [file omitted_proofs.tex]

\section{Omitted Proofs}\label{app:proofs}

In this section, we present the missing proofs of several technical results from the main text.

\subsection{Proof of Lemma~\ref{lem:de_simple} (Doubly Exponential Error Blowup)}

We prove Lemma~\ref{lem:de_simple} by explicitly constructing an MDP exhibiting the doubly exponential blow-up.

Recall that $S=A=\{1,2\}$. We define the reward function as $R_h(s,a) = 0$ for all $(s,a, h) \in S \times A \times [H-1]$ with terminal reward $R_H(s,a) = 1/2$ for all $(s,a) \in S \times A$. The transition kernel is
\[
P_h(\cdot|s,a) = \begin{cases}
\delta_s, & \text{ if } s = a, \\
\mathrm{uniform}(S), & \text{ if } s \neq a
\end{cases} \qquad \forall h \in [H],
\]
where $\delta_s$ denotes the Dirac distribution at $s$. We remark that all policies are optimal with value and action-value functions
\[
Q^*_h(s,a) = V^*_h(s) = \frac{1}{2}, \qquad \forall (s,a,h) \in S\times A \times [H].
\]
Consider policy evaluation for one of the optimal policies, $\pi = \{\pi_h\}_{h \in [H]}$, where for all $h \in [H]$, 
\[
\pi_h(s) \coloneqq \begin{cases}
1, & \text{ if } s = 1,\\
2, & \text{ if } s = 2.
\end{cases}
\]
For $h=H-1, \ldots, 1$, we use the algorithm described in Section~\ref{sec:double_exp} to  compute the estimates $\hat{Q}^\pi_h \in \mathbb{R}^{2\times2}$ and $\hat{V}^\pi_h \in \mathbb{R}^{2}$  of the value and action-value functions of $\pi$. For this algorithm, we note that a global optimum $(u,v)$ of the least-squares formulation~\eqref{eq:least_squares} is 
\begin{equation*}
u_1 = v_1 = \sqrt{\hat{Q}^\pi_h(1,1)}, 
\quad 
u_2 = \frac{\hat{Q}^\pi_h(2,1)}{\sqrt{\hat{Q}^\pi_h(1,1)}},
\quad\text{and}\quad 
v_2 = \frac{\hat{Q}^\pi_h(1,2)}{\sqrt{\hat{Q}^\pi_h(1,1)}},
\end{equation*}
which leads to formula for $\hat{Q}^\pi_h(2,2)$ given in Equation~\eqref{eq:est}.

We state a lemma that shows if our estimate at step $h+1$ is not perfect, then the error at step $h$ increases quadratically.

\begin{lemma}\label{lem:ex}
Let $\pi$ and the MDP be defined as above. For each $h \in [H-1]$, suppose that the value function estimate of $V^\pi_{h+1}$ is in the form
\[
\hat{V}^\pi_{h+1} = \begin{bmatrix}
\frac{1}{2}\\
\frac{1}{2} + 2 \eps_{h+1}
\end{bmatrix}.
\]
Then the algorithm described in Section~\ref{sec:double_exp} results in the estimate
\[
\hat{V}^\pi_{h} = \begin{bmatrix}
\frac{1}{2}\\
\frac{1}{2} + 2 \eps_{h}
\end{bmatrix}
\]
where $\eps_h = \eps_{h+1} + \eps_{h+1}^2$.
\end{lemma}
\begin{proof}[Proof of Lemma \ref{lem:ex}]
We compute the first row and column of $\hat{Q}^\pi_h$ using the exact Bellman operator given $\hat{V}^\pi_{h+1}$:
\begin{align*}
  \hat{Q}^\pi_h(1, 1) &=  R_h(1,1) + \sum_{s' = 1}^2 P_h(s'| 1, 1)\hat{V}^\pi_{h+1}(s')=  \hat{V}^\pi_{h+1}(1) = \frac{1}{2},\\
  \hat{Q}^\pi_h(1, 2) &=  R_h(1,2) + \sum_{s' = 1}^2 P_h(s'| 1, 2) \hat{V}^\pi_{h+1}(s')=  \frac{1}{2}(\hat{V}^\pi_{h+1}(1) + \hat{V}^\pi_{h+1}(2)) = \frac{1}{2} + \eps_{h+1},\\
  \hat{Q}^\pi_h(2, 1) &=  R_h(2,1) + \sum_{s' = 1}^2 P_h(s'|  2, 1) \hat{V}^\pi_{h+1}(s')=  \frac{1}{2}(\hat{V}^\pi_{h+1}(1) + \hat{V}^\pi_{h+1}(2) )= \frac{1}{2} + \eps_{h+1}.
\end{align*}
Using the estimator in Equation \eqref{eq:est} to compute $\hat{Q}^\pi_h(2,2)$:
\[
\hat{Q}^\pi_h(2,2) = \frac{\hat{Q}^\pi_h(1,2)\hat{Q}^\pi_h(2, 1) }{\hat{Q}^\pi_h(1,1)} = \frac{1}{2} + 2(\eps_{h+1} + \eps_{h+1}^2).
\]
Hence, following policy $\pi_h$ results in the value function estimate: 
\[
\hat{V}^\pi_{h} = \begin{bmatrix}
\frac{1}{2}\\
\frac{1}{2} + 2 \eps_{h}
\end{bmatrix}
\]
for $\eps_h = \eps_{h+1} + \eps_{h+1}^2$. 
\end{proof}

Using Lemma~\ref{lem:ex}, we can show that if the estimate for the terminal value function $V^\pi_H$ is not be perfect, then the estimation error blows up quickly as we recurse backward to compute an estimate of $V^\pi_1$. In particular, we establish the following lemma, which immediately implies the desired Lemma~\ref{lem:de_simple}.

\begin{lemma}[Doubly Exponential Growth]\label{lem:de}
Let $\pi$ and the MDP be defined as above. Suppose that the estimate for the terminal value function is of the form 
\[
\hat{V}^\pi_{H} = \begin{bmatrix}
\frac{1}{2}\\
\frac{1}{2} + 2 \eps_{H}
\end{bmatrix}
\]
for some $\eps_{H}\in o(1)$.
Then, the algorithm described in Section~\ref{sec:double_exp} results in the estimate
\[
\hat{V}^\pi_{1} = \begin{bmatrix}
\frac{1}{2}\\
\frac{1}{2} + \Omega\left(\left((1+ \eps_H)^{c'}\right)^{2^{H - \frac{\ln(1/\eps_H)}{\ln(1+\eps_H)} - 1 - c'}}\right)
\end{bmatrix}
\]
for $H > 1 + \frac{\ln(1/\eps_H)}{\ln(1+\eps_H)} + c'$ and $c' = \left\lceil \frac{\ln(1/\eps_H)}{\ln(1+\eps_H)}\right\rceil - \frac{\ln(1/\eps_H)}{\ln(1+\eps_H)}$.
\end{lemma}

\begin{proof}[Proof of Lemma \ref{lem:de}]
Let $H > 1 +\left\lceil \frac{\ln(1/\eps_H)}{\ln(1+\eps_H)}\right\rceil, c' = \left\lceil \frac{\ln(1/\eps_H)}{\ln(1+\eps_H)}\right\rceil -  \frac{\ln(1/\eps_H)}{\ln(1+\eps_H)},$ and $t = H - 1 - \frac{\ln(1/\eps_H)}{\ln(1+\eps_H)} - c'$.
Recursively applying Lemma \ref{lem:ex} gives:
\[
\hat{V}^\pi_{t} = \begin{bmatrix}
\frac{1}{2}\\
\frac{1}{2} + 2\eps_t
\end{bmatrix}
\]
where $\eps_h = \eps_{h+1}(1 + \eps_{h+1})$ for $h \in \{t, \ldots, H-1\}$. Since $\eps_h > \eps_{h+1}$, it follows that $\eps_h > (1 + \eps_H)\eps_{h+1}$ for $h \in [H]$. Thus, $\eps_t > (1+ \eps_H)^{H-t-1}\eps_H$. Plugging in the value for $t$ gives
\[
\eps_t > (1+ \eps_H)^{\frac{\ln(1/\eps_H)}{\ln(1+\eps_H)} + c'}\eps_H = (1+ \eps_H)^{c'}.
\]
Recursively applying Lemma \ref{lem:ex} again gives:
\[
\hat{V}^\pi_{1} = \begin{bmatrix}
\frac{1}{2}\\
\frac{1}{2} + 2\eps_1
\end{bmatrix}
\]
where $\eps_h = \eps_{h+1} + \eps_{h+1}^2$ for $h \in [t-1]$. Lower bounding $\eps_1$ it terms of $\eps_t = (1 + \eps_H)^{c'}$ gives
\[
\hat{V}^\pi_{1} = \begin{bmatrix}
\frac{1}{2}\\
\frac{1}{2} + \Theta \left(\eps_t^{2^t} \right)
\end{bmatrix}.
\]
Using the lower bound on $\eps_t$ and plugging in our value for $t$ proves the lemma. 
\end{proof}

We make a slight modification to the MDP to show that policy evaluation of a near optimal policy results in exponential growth even for very small $\eps$, e.g., $\eps \ll 1/H$. We use the same setup except for some positive constant $\alpha$, we change the reward function to be  \[R_h(s,a) = \begin{bmatrix} 0 & \alpha - \frac12(\alpha^2 + 1) \\
\alpha - \frac12(\alpha^2 + 1) & 0
\end{bmatrix}\]
for all $(s,a, h) \in S \times A \times [H-1]$ with terminal reward 
\[R_H(s,a) = \begin{bmatrix} \alpha^2 \\
1
\end{bmatrix}\]
for all $(s,a) \in S \times A$. The policy defined above, 
\[
\pi_h(s) \coloneqq \begin{cases}
1, & \text{ if } s = 1,\\
2, & \text{ if } s = 2,
\end{cases}
\]
for all $h \in [H]$, is not optimal as the optimal action depends on $\alpha$. In our case, setting $\alpha = 1/2$ clearly results in $\pi$ being sub optimal. It follows from this policy that 
\[
Q^{\pi}_h(s,a) = \begin{bmatrix} \alpha^2 & \alpha \\
\alpha & 1
\end{bmatrix},
V^{\pi}_h(s) = \begin{bmatrix} \alpha^2 \\
1
\end{bmatrix}, \qquad \forall (s,a,h) \in S\times A \times [H].
\]
Following the same setup as the doubly exponential result, for $h=H-1, \ldots, 1$, we use the algorithm described in Section~\ref{sec:double_exp} to  compute the estimates $\hat{Q}^\pi_h \in \mathbb{R}^{2\times2}$ and $\hat{V}^\pi_h \in \mathbb{R}^{2}$  of the value and action-value functions of $\pi$. 

\begin{lemma}\label{lem:ex2}
Let $\pi$ and the MDP be defined as above. For each $h \in [H-1]$, suppose that the value function estimate of $V^\pi_{h+1}$ is in the form
\[
\hat{V}^\pi_{h+1} = \begin{bmatrix}
\frac{1}{4}\\
1 +  \eps_{h+1}
\end{bmatrix}.
\]
Then the algorithm described in Section~\ref{sec:double_exp} results in the estimate
\[
\hat{V}^\pi_{h} = \begin{bmatrix}
\frac{1}{4}\\
1 +  \eps_{h}
\end{bmatrix}
\]
where $\eps_h > 2 \eps_{h+1}$.
\end{lemma}
\begin{proof}[Proof of Lemma \ref{lem:ex2}]
Using the same steps as the proof of the previous lemma, it follows that 
\[\hat{Q}_{h} = \begin{bmatrix} \frac{1}{4} & \frac{1}{2} + \frac{\eps_{h+1}}{2} \\
\frac{1}{2} + \frac{\eps_{h+1}}{2} & 1 + 2\eps_{h+1} + \eps_{h+1}^2
\end{bmatrix},
\] 
where $\hat{Q}_h(2, 2) = \hat{Q}_h(1, 2) \hat{Q}_h(2, 1) /\hat{Q}_h(1, 1) $. It follows from the definition of the value function of the defined policy that 
\[\hat{V}_{h} = \begin{bmatrix} \frac{1}{4} \\
1 + \eps_{h+1}(2 + \eps_{h+1})
\end{bmatrix}.
\]
Since $\eps_{h+1} > 0$, it follows that $\hat{V}_{h} = 1 + \eps_h$ for $\eps_h > 2 \eps_{h+1}$
\end{proof}
With the recurrence relation $\eps_h > 2 \eps_{h+1}$, it follows that the error from policy evaluation grows exponentially with respect to $H$ even for small $\eps_H$, i.e., repeatedly apply the above lemma results in $\hat{V}_1^\pi(2) = 1+ \eps_H 2^{H-1}$.

\subsection{Proof of Proposition \ref{prop:lrEst}}
\label{sec:proof_lrEst}

We next present the proof of Proposition \ref{prop:lrEst}, which shows  that if the reward function and transition kernel are low rank, then for any value function estimate $\hat{V}_{h+1}$, $r_h + [P_h\hat{V}_{h+1}]$ has rank upper bounded by $d$.

\begin{proof}[Proof of Proposition \ref{prop:lrEst}]
Let MDP $M = (S,A,P,r, H)$ satisfy Assumption \ref{asm:lrtk} (specifically, $P_h$ has Tucker rank $(|S|, |S|, d)$. It follows that for each $h \in [H]$, there exists an $|S| \times |S| \times d$ tensor $U^{(h)}$, an $|A| \times d$ matrix $V^{(h)}$, and an $|S| \times d$ matrix $W^{(h)}$ such that
\[
P_h(s'|s,a) = \sum_{i=1}^d U^{(h)}_{s', s, i}V^{(h)}_{a, i} \quad\text{ and }\quad r_h(s,a) = \sum_{i=1}^d W^{(h)}_{s, i}V^{(h)}_{a, i}.
\]
Hence, for any value function estimate $\hat{V}_{h+1}$,
\begin{align*}
    r_h(s,a) + P_h \hat{V}_{h+1} &= \sum_{i=1}^d W^{(h)}_{s, i}V^{(h)}_{a, i} + \sum_{s' \in S}\hat{V}_{h+1}(s')P_h(s'|s,a)\\
    &=\sum_{i=1}^d W^{(h)}_{s, i}V^{(h)}_{a, i} + \sum_{s' \in S}\hat{V}_{h+1}(s')\sum_{i=1}^d U^{(h)}_{s', s, i}V^{(h)}_{a, i} \\
    &= \sum_{i=1}^d V^{(h)}_{a, i} \left (W^{(h)}_{s, i}  + \sum_{s' \in S}\hat{V}_{h+1}(s') U^{(h)}_{s', s, i} \right).
\end{align*}
Since $W^{(h)}_{:, :}  + \sum_{s' \in S}\hat{V}_{h+1}(s') U^{(h)}_{s', :, :}$ is an $|S|\times d$ matrix, $r_h(s,a) + P_h \hat{V}_{h+1}$ has rank at most $d$. The same result holds when $P_h$ has Tucker rank $(|S|, d, |A|)$ from a similar argument.
\end{proof}
