# Supplementary material for: Overcoming the Long Horizon Barrier for Sample-Efficient Reinforcement Learning with Latent Low-Rank Structure
Source: arXiv:2206.03569 source file (2023-06-09)
Supplement: Supplementary file 7 [file rebuttal.tex]

\section{Response to Reviewers}

We appreciate the reviewer’s feedback and suggestions, and have incorporated the below discussion into our revision. We first summarize the major edits in the new revision:
\begin{itemize}
    \item Included numerical experiments benchmarking the performance of two variants of our algorithms LR-MCPI and LR-EVI, one using the matrix estimation algorithm from \cite{serl}, and another using \texttt{Soft-Impute} from \cite{softImpute}. We compare against vanilla Empirical Value Iteration and Monte Carlo Policy Iteration, to clearly show the difference between using low rank matrix estimation as opposed to the standard RL algorithm. We chose a MDP which is in fact full rank, but the spectrum decays so quickly so that it is approximately low rank. This illustrates the robustness of the algorithm when the rank is not known (or even full rank). See Section 8 for the experiments, and Section D in the appendix for details regarding hyperparameter tuning.
    \item We added an explicit discussion of how approximate low rank structure and incoherence could arise naturally in MDPs, see the end of Section 5.
    \item We added a discussion of the optimality of our results with respect to different parameters in section 7.1, and we added a discussion in the paragraph prior about the comparison between our impossibility results in Theorem 2 and our upper bound results in Theorems 7-9.
    \item We added clarifications of reviewer questions throughout the paper, including clarifications of steps in the proof sketch, and clarification about the information theoretic setup for the impossibility results in Theorem 2.
    \item We moved the extensions to continuous state and actions spaces and using existing matrix estimation algorithms to the appendix as suggested by reviewers.
\end{itemize}

The two major requests for the one-shot revision were to include numerical experiments and to address concerns about clarity of presentation raised by the reviewers. We first detail our revisions regarding these two requests, followed by a detailed response to individual questions from reviewers.

\medskip \noindent
{\bf Numerical Experiments:} We agree with all the reviewers that our paper can be improved by adding numerical experiments that empirically validate our two algorithms' theoretical benefits. In Section \ref{sec:experiments}, we add experiments that benchmark our low rank algorithms against vanilla Empirical Value Iteration and Monte Carlo Policy Iteration. We construct an MDP motivated by the Oil Discovery problem, which we choose due to an ease of explaining the low rank structure in the problem. The transition kernel is low rank, yet we choose a reward function that is only approximately low rank, despite actually being full rank. This was chosen to illustrate the robustness of our algorithm as it is not obvious what "rank" should be used to tune parameters in the algorihm (this is a specific request from the reviewers). 

The rank parameter is only used in the algorithm to choose the sampling probabilities, $p_S$ and $p_A$ if using the matrix estimation algorithm from \cite{serl}, or $p_{SI}$ if using \texttt{Soft-Impute} from \cite{softImpute}. As a result, to test for robustness to the knowledge of rank, we include tables in the appendix section D.3 that show performance of the low rank algorithms for different choices of $p_S$, $p_A$, and $p_{SI}$. We find that while the performance can change with different values of $p_S$, $p_A$, and $p_{SI}$, the difference in performance is not significant, suggesting that the algorithm is fairly stable with respect to the choice of these parameters and thus also does not require precise knowledge of the rank. 

The optimal $Q_1^*$ function ranges in value from roughly 8.3 to 9.6, thus an entrywise error of 0.8 would translate to roughly 10\% error.
Our results show that the sample complexity of finding a near-optimal $Q$ function using LR-EVI and LR-EVI $+$ \texttt{SI} is significantly lower compared to vanilla Empirical Value Iteration (EVI). Similarly, the sample complexity of finding a near-optimal $Q$ function using LR-MCPI and LR-MCPI $+$ \texttt{SI} is much lower than vanilla Monte Carlo Policy Iteration (MCPI). Furthermore, we show that when we fix the budget of samples collected, the low-rank algorithms learn significantly better $Q$ functions compared to Empirical Value Iteration and Monte Carlo Policy Iteration. Most compelling is that even when there are insufficient samples for EVI or MCPI to even produce any estimate at all (i.e. insufficient to sample even once from each state-action pair), the low rank algorithms can still produce reasonable estimates. 



\medskip \noindent
{\bf Improved Presentation:} We have fixed the notational errors and typos pointed out by the reviewers (thanks!). We have added missing definitions of the Tucker rank, and have improved the presentation of the information theoretic lower bound to address reviewer concerns and questions. We have also added references for the definition of a $\mu$-incoherent matrix along with a discussion of how incoherence could naturally arise, and we have added some explanation of the key steps of the proof of Lemma \ref{lem:ME_error_amplification}. 

\medskip \noindent
Below, we respond in details to the comments from each reviewr. 

\medskip \noindent
{\bf Reviewer A:}
\begin{itemize}
  \setlength\itemsep{.3em}
    \item {\em In the abstract, at first glance, the negative result seems to contradict to the positive result. The authors should point out that the positive result is derived under additional assumptions than just assuming low rank.}
    
    Thanks! we have now clarified that. 

    \item {\em The paper would be improved by presenting a concrete practical example (with explicitly given state-action space, low-rank structure, and anchor states and actions) to demonstrate the applicability of the results.}

    Thanks for the suggestion. We have included experiments in Section \ref{sec:experiments} on a concrete MDP motivated by the Oil Discovery problem. We sample anchor states and actions at random, and we also discuss the low rank structure of the MDP. In particular our chosen MDP has low rank transition kernel, yet only approximately low rank reward function. Our numerical results showing the improved efficiency of our low-rank algorithms on this instance. 

    \item  {\em From my understanding, to implement the algorithm it is crucially important that the agent can sample a transition at any specific state-action pair. Therefore, it seems that even in principle the algorithm cannot be generalized to the setting where the samples are coming from a Markovian trajectory.}

    Indeed, this is a good observation, and it is an interesting future direction to figure out how to extend our results to a setting in which the samples can only come from a Markovian trajectory. This would take more innovation in the matrix estimation literature as there is limited results that can handle arbitrary sampling patterns. We have commented on this as a future direction in our conclusion.

    \item  {\em There seems to be a large gap between the sample complexity dependence on H and the lower bound. Is it an artifact of the proof? Are additional assumptions, or different algorithms, needed to match the lower bound?}

    \tsedit{Our dependence on the horizon $H$ is fairly standard as it matches the dependence on $H$ for vanilla $Q$-value iteration. However, there is a gap between our upper bounds and the $H^3$ lower bound in Lemma~\ref{lem:lrlb}, which is proven for homogeneous MDPs while our algorithm allows for nonhomogenous rewards and transition kernels. Reducing the dependence to $H^4$ would likely require the total variance technique from \cite{sidford2019nearoptimal}, which requires estimates of the variance of the policy at a given state-action pair. One can show that the variance of the Bellman operator is low rank under the strongest assumption of a low Tucker rank transition kernel, but the corresponding rank of the matrix of variances is $O(d^2)$. Hence, while it may be possible to adapt this variance technique to achieve the optimal dependence on $H$ in our low-rank settings, doing so may incur a significantly worse dependence on $d$, i.e., $d^{6}$. } We have added a discussion on the suboptimality of our algorithms' dependence on $H$ and $d$ in Section 7.1.
\end{itemize}




\medskip \noindent
{\bf Reviewer B:}
\begin{itemize}
  \setlength\itemsep{.3em}
    \item {\em While the presence of a low-rank structure is plausible for typical problem instances, it's not clear to me how one can be sure of that in a particular problem instance, let alone how one would know the value of the rank, and in that sense the practical merit of the proposed algorithm is unfortunately not so evident. The complete lack of any numerical experiments is also somewhat disappointing and reinforces the latter concern.}

We include a discussion at the end of Section 5 regarding how low rank structure can naturally arise from settings in which the tabular MDP well approximates a continuous MDP with smoothness properties (either because it was derived by discretizing a continuous MDP or it represents a very large population of states/actions that can be approximated by a continuous population distribution). In these settings, the MDP will satisfy our approximately low rank conditions. In Section \ref{sec:approx} we present results showing that LR-EVI is robust to the low-rank approximation error. We also show empirically that both of our low-rank RL algorithms work well on an approximately low-rank MDP (where the MDP actually has full rank). See Section \ref{sec:experiments} for our numerical experiments.
    
Regarding knowing the rank parameter to implement the algorithms, it turns out that our algorithm is not very sensitive to the precise knowledge of the rank. In our low-rank RL algorithms, the rank parameter is only used to choose the observation probabilities, i.e., $p_S$ and $p_A$, which are the probability that each state or action is included in the respective anchor set. Hence if we show the algorithm is robust to the choice of $p_S$ and $p_A$, it also implies our algorithm is robust to the choice of the rank parameter in the algorithm. In Section D.3 of the appendix, we show the performance of our algorithm on varying values of $p_S$ and $p_A$, considering $p_S = p_A = p \in [ 0.025, 0.05, 0.075, 0.1]$. The magnitude of the $Q^*_1$ entries range from 8.3 to 9.6, and the errors for different choices of $p$ only differed by around $0.06$, suggesting that the algorithm is fairly stable and robust to the particular choice of $p$. One could also empirically use cross validation to choose $p$, or simply choose $p$ to be as large as possible given specified computational and memory limits.

We also comment that the question of tuning the rank parameter of a low rank matrix estimation algorithm is universal to the all proposed algorithms in the matrix estimation literature. \tsreplace{For example, the }{For example, Universal Singular Value Thresholding (USVT) requires a user to choose $\eta$, the singular value thresholding constant, that balances computational speed and performance, i.e., the theoretical error bounds worsen as $\eta \to 0$ \cite{Chatterjee_2015}. \cite{Chatterjee_2015} found that in practice setting $\eta$ to be a small constant, $\eta = 0.01$, yielded good results. Similarly, the} algorithm Singular Value Planning presented in \cite{Yang2020Harnessing} \tsedit{requires knowledge of the rank to choose observation probability, $p_{SI}$, for their \texttt{Soft-Impute} step. To resolve this issue, \cite{Yang2020Harnessing} observed that their algorithm performs well for a range of $p_{SI}$; setting $p_{SI}$ to be $0.2$ and $0.6$ yielded similar results, so they concluded it suffices to choose $p_{SI} = 0.2$.} 

    \item {\em The relation between a low-dimensional structure (of the Q-function presumably) and the state space collapse phenomenon for queueing systems sounds interesting, but might be worth elaborating on a bit further.}

    We intended that example to illustrate that there are scenarios in which a low dimensional structure can arise under optimal policies though not under suboptimal policies. However, as that connection is not very formal to our MDP setup and could be more confusing than illuminating, we have removed this comment.
    
    \item {\em The definition of the Q-function in Equation (2) looks a bit suspicious to me.}

    Sorry, we did have a typo there. We have fixed our definition of the $Q$-function \tsedit{with the new version as,
    \[
    Q_h^\pi(s, a) := \E\left[ \left. \textstyle  \sum_{t = h}^H r_t(s_t, a_t) ~\right|~ s_h = s, a_h = a \right]
    \]
    where $a_t \sim \pi_t(s_t)$ and $s_{t+1} \sim P_{t}( \cdot | s_{t},a_{t})$.} Thanks!

    \item {\em The a in the second part of Equation (6) is notationally overloaded.}

    Thanks for pointing this out, it is now fixed.

    \item {\em It may not hurt to provide references for non-standard concepts like the matrix Bernstein inequality and the Courant-Fischer minimax theorem.}

    We have added citations for the matrix Bernstein inequality and the singular value Courant-Fischer Minimax Theorem in section \ref{sec:proofSketch}. We also present both of those theorems in addition to Hoeffding's inequality and one-sided Bernstein's inequality in appendix \ref{sec:additional_theorems}.
\end{itemize}


\medskip \noindent
{\bf Reviewer C:}
\begin{itemize}
  \setlength\itemsep{.3em}
    \item {\em In my view, the contribution of Section 8 is not significant, or in other words, given the space constraint, having a numerical section illustrating the performance of the algorithm in some concrete problems would have been more a more interesting addition.}

    We have moved the extensions to the continuous state and action space setting to the appendix and have added a numerical section illustrating the improved efficiency of our low-rank RL algorithms (see Section \ref{sec:experiments}).

    \item {\em I did not understand the description of the two MDPs prior to Lemma 1. For instance, why there is an initial step $h = 0$ where $r_0^\theta(s_0,a)=0$? As a consequence, the whole presentation in this section was confusing.}

    Sorry for the inconsistent notation. We have now relabeled the initial step as $h = 1$ instead of $h = 0$. We have fixed the notation and analysis to be consistent with the notation introduced in the Preliminaries section. 

    \item {\em In the proof of Theorem 2 (end of page 7), what is the meaning of 1/4-suboptimal? The notion of suboptimality gap seems to be defined for the first time at the end of page 8.}

    \tsedit{We have edited that section to avoid using that unclear language. We now directly explain what we meant `` If $\theta = \theta_1$ and action 2 is taken instead, $\pi_1(s_0)=2$, then the policy incurs a $1/4$ penalty relative to the optimal policy. If $\theta = \theta_2$ and action $1$ is taken, $\pi_1(s_0) = 1$, then the policy incurs a $5/4$ penalty relative to the optimal policy.''}
    

    \item {\em Assumption 4, what is Tucker rank?}

    Thank you for pointing out that we forgot to define Tucker rank. We provide the following definition of the Tucker rank of a tensor. 
    \tsreplace{
    \begin{definition}[Tucker Rank \cite{tucker}]
The Tucker decomposition of a tensor $X\in\R^{n_1 \times n_2 \times \ldots \times n_m}$ is
\[
X = G \times_1 A_1 \times_2 A_2 \ldots \times_m A_m
\]
where $G \in \R^{d_1 \times d_2 \times \ldots \times d_m}$, $\times_i$ denotes the $i$-mode product (defined in the notation paragraph in section \ref{sec:prelim}), and $A_i \in \R^{n_i \times d_i}$ are matrices with orthonormal columns for all $i \in [m]$. Then, we define the Tucker rank of $X$ as $(d_1, d_2, \ldots, d_m)$.
\end{definition}}{
\begin{definition}[Tucker Rank \cite{tucker}]
The Tucker rank of a tensor $X \in \R^{n_1\times n_2 \times n3}$ is the smallest $(d_1, d_2, d_3)$ such that there exists a core tensor $G \in \R^{d_1 \times d_2 \times d_3}$ and orthonormal latent factor matrices $A_i \in \R^{n_i \times d_i}$ for $i \in [3]$ such that for all $(a,b,c) \in [n_1]\times[n_2]\times[n_3]$,
\[X(a,b,c) = \sum_{\ell_1 \in [d_1]} \sum_{\ell_2 \in [d_2]} \sum_{\ell_3 \in [d_3]} G(\ell_1,\ell_2,\ell_3) A_1(a,\ell_1) A_2(b,\ell_2) A_3(c,\ell_3)\]
\end{definition}}

\item {\em On page 12 in step 2, the notation ME() is used without explanation. This is explained in the section 6.2 for the first time.}

We have added to the first sentence of Section 6.1 ``We present two Low Rank RL algorithms, which take as input any matrix estimation algorithm, \texttt{ME}$(\cdot)$, \tsedit{that takes in a subset of entries of the matrix and returns an estimate of the whole matrix}''. Thus \texttt{ME}$(\cdot)$ is simply a matrix estimation subroutine taken as input to the algorithm.


\item {\em After equation (7), what does it mean that $Q_h$ is $\mu$-incoherent?}

A matrix $Q \in \R^{|S| \times |A|}$ with singular value decomposition $Q = U\Sigma V^\top$, $U\in\R^{|S|\times d}$, and $V\in\R^{|A|\times d}$ is $\mu$-incoherent if $ \max_{i \in [|S|]} \|U_{i}\|_2 \leq \sqrt{\mu d/|S|}$ and $ \max_{j \in [|A|]} \|V_{j}\|_2 \leq \sqrt{\mu d/|A|}$, where $U_i$ denotes the $i$-th row of a matrix $U$. See Section \ref{sec:asm} for the definition (Definition \ref{asm:inco}) and discussion of why this property is necessary for our approach. We have included a reference to the location of the definition after Equation (7). 

\item {\em Proof of Lemma 11 on page 15, how is the inequality derived?}

We have included a couple of more steps to give intuition on how the inequality is derived (see Section \ref{sec:proofSketch}).
\begin{align*}
\left|\bar{Q}_h(s,a) - Q_h(s,a)\right| 
&\lesssim \left \|[\hat{Q}_h(S^\#, A^\#)]^\dagger \right\|_{op} ~~\cdot~~\left \|\hat{Q}_h(S^\#, a)\hat{Q}_h(s, A^\#) - Q_h(S^\#, a)Q_h(s, A^\#)   \right \|_F\\
&+
\left\| \left[ \hat{Q}_h(S^{\#},A^{\#})\right]^{\dagger} - \left[ Q_h(S^{\#},A^{\#})\right]^{\dagger} \right\|_{op} ~~\cdot~~
\left\|Q_h(S^{\#}, a) Q_h(s, A^{\#})\right\|_F
\end{align*}
This step is a result of applying the triangle inequality and using the operator norm since for any rank $d$ matrix $Q$ with $(k, \alpha)$-anchor states and actions, for all $(s, a) \in S\times A$, $Q(s, a) = Q(s, A^\#) [Q(S^\#, A^\#)]^\dagger Q(S^\#, a) $. The second step uses perturbation results of pseudoinverses and bounds due to $Q_h(s, a)$ being bounded. 
\begin{align*}
\left|\bar{Q}_h(s,a) - Q_h(s,a)\right| 
&\lesssim \left(\frac{1}{\sigma_d(Q_h(S^{\#},A^{\#})))} \right)~~\cdot~~ k \|Q_h\|_{\infty}(2\eta + \eta^2) \\
&+ \left( \frac{\eta^{\#} k}{(\sigma_d(Q_h(S^{\#},A^{\#})))^2}\right) ~~\cdot~~ \|Q_h\|^2_{\infty} k = O(\alpha k \eta + \alpha^2 k^2 \eta^{\#}).
\end{align*}

\item {\em Equation (7). How can the function $Q$ be estimated for all pairs $(s, a)$ if the right hand-side is only known for the pairs $(s,a)$ in the subset $\Omega_h$?}

This point is the strength of matrix estimation methods and why we use it in LR-EVI and LR-MCPI to improve upon standard RL algorithms. The matrix estimation literature focuses on recovering the missing entries of a partially observed low-rank matrix with noise ($\Omega$ refers to the set of indices of the observed entries). The main challenge in matrix estimation is balancing how many entries one is required to observe (the size of $\Omega$) and the noise of the observed entries to get the desired error guarantees of the fully recovered matrix. 

A low-rank (rank-$d$) $|S|$-by-$|A|$ matrix has $d(|S|+|A|)$ degrees of freedom compared to $|S||A|$ in general. Thus, we use matrix estimation to exploit the low-rank structure to recover the whole matrix while only observing a number of entries that scales with $|S|+|A|$ instead of $|S||A|$. See the second paragraph of the \textit{MDPs with Low Rank Structure} section in Section \ref{sec:introduction}.

The matrix estimation method used in LR-EVI and LR-MCPI is the one introduced in \cite{serl}. The main intuition behind that method is that for any rank $d$ matrix $Q$ with $(k, \alpha)$-anchor states and actions, $S^{\#}$ and $A^{\#}$, for all $(s, a) \in S \times A$,
\[
Q(s, a) = Q(s, A^{\#})[Q(S^\#, A^\#)]^\dagger Q(S^\#, a).
\]
Thus, we can recreate the original matrix by observing only specific rows and columns of $Q$, see Figure~\ref{fig:anchor_sets}.
\begin{figure}[H]
    \centering
    \includegraphics[width = .25\textwidth]{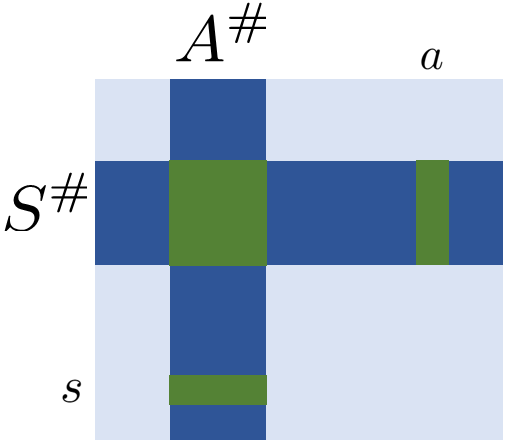}
    \caption{Estimating $Q(s, a)$, the black square, using entries from only specific rows and columns, the green entries ($Q(s, A^{\#}), Q(S^\#, A^\#),$ and $ Q(S^\#, a)$). The dark blue corresponds to the anchor state and actions rows and columns.}
    \label{fig:anchor_sets}
\end{figure}
Thus, for this method, the number of observed entries, $\Omega_h$, scales with $|\Omega_h| \in \Tilde{O}(\mu d(|S|+|A|))$, where $Q$ is $\mu$-incoherent. In general, without the low-rank assumption, one needs to observe all the entries of the matrix. 

Thus, under certain low-rank structure, i.e., Assumptions \ref{asm:lrqt}, \ref{asm:lrqe}, or \ref{asm:lrtk}, we can control the noise on those observed entries with concentration inequalities, and our algorithms learn an $\eps$-optimal policy with a sample complexity that scales with the sum of the size of the state and action spaces instead of the product, $|S|+|A|$ vs. $|S||A|$. 


\end{itemize}
% We thank Reviewer C for pointing out places in our paper that lacked sufficient introduction or explanation, and we have addressed those issues. We have added a sentence to the beginning of Section \ref{sec:algoStatement} that defines $\texttt{ME}(\cdot)$ as the matrix estimation method that is given to our algorithm. To address the question ``how can the function $Q$ be estimated for all pairs $(s, a)$ if the right hand-side is only known for the pairs $(s, a) \in \Omega_h$,'' we realize that the main intuition behind our results in this paper were not explained well enough. For a general MDP, to learn an $\eps$-optimal policy, one must incur a sample complexity that depends on the product of the size of the state and action spaces, $|S||A|$. However, under certain low-rank structure, Assumptions \ref{asm:lrqt}, \ref{asm:lrqe}, or \ref{asm:lrtk}, our algorithms learn an $\eps$-optimal policy with a sample complexity that scales with the sum of the size of the state and action spaces instead of the product, $|S|+|A|$ vs. $|S||A|$. The intuition behind this approach is that if $Q_h$ is a low-rank matrix, the degrees of freedom are reduced from $|S||A|$ (for a general matrix with dimension $|S|$ by $|A|$, to $d(|S|+|A|)$, where $d$ is the rank of the matrix. Thus, by using low-rank matrix estimation methods, our algorithms admit those improved sample complexities. 

% To explain our chosen matrix estimation method, from Lemma 12 in \cite{serl}, we have that for any rank $d$ matrix $Q$ with $(k, \alpha)$-anchor states and actions, $S^{\#}$ and $A^{\#}$, for all $(s, a) \in S \times A$,
% \[
% Q(s, a) = Q(s, A^{\#})[Q(S^\#, A^\#)]^\dagger Q(S^\#, a).
% \]
% Thus, we can recreate the original matrix with knowledge of only specific rows and columns of $Q$, see Figure~\ref{fig:anchor_sets}.
% \begin{figure}[H]
%     \centering
%     \includegraphics[width = .5\textwidth]{img/anchor.PNG}
%     \caption{Estimating $Q(s, a)$, the black square, using entries from only specific rows and columns, the green entries ($Q(s, A^{\#}), Q(S^\#, A^\#),$ and $ Q(S^\#, a)$). The dark blue corresponds to the anchor state and actions rows and columns.}
%     \label{fig:anchor_sets}
% \end{figure}

% With this method, we can upper bound the error of our estimate of each entry of the whole matrix provided that the estimation error of the entries in $\Omega$ is small enough. Under standard matrix estimation assumption, incoherence and bounded condition number, we show that $\Omega \in \Tilde{O}(d)$ is large enough to learn an $\eps$-optimal policy. Hence, using this matrix estimation method, we reduce the sample complexity from $|S||A|$ to $\mathrm{poly}(d)(|S|+|A|)$.
